# Supplementary material for: Electron-boson spectral density functions of cuprates obtained from optical spectra via machine learning
Source: arXiv:2106.04162 source file (2021-12-14)
Supplement: Supplementary file 1 [file Supplementary_JH_1a.pdf]

## Supplementary Materials

### Glue functions of cuprates obtained from optical spectra via machine learning

Hwiwoo Park<sup>1</sup>, Jun H. Park<sup>2</sup>, and Jungseek Hwang<sup>1</sup>

<sup>1</sup>Department of Physics, Sungkyunkwan University, Suwon, Gyeonggi-do 16419, Republic of Korea

<sup>2</sup>School of Mechanical Engineering, Sungkyunkwan University, Suwon, Gyeonggi-do 16419, Republic of Korea

#### The convolutional neural network (CNN)

The convolutional neural network (CNN) is the most common and popular deep learning method. It is well known for its remarkable successes in image classification problems. Fig. S1 shows a schematic neural network structure of CNN. The convolutional layer converts the input data into a collection of batches. The pooling layer collects the maximum value of each batch from the convolutional layer. The convolutional and pooling layers are repeatedly applied in the model, where we have used four pairs of them. The flatten layer changes the dimension of resulting data to one dimensional array. The dense layer is fully connected with the flatten layer and makes them matched with the dimension of the output data. Comparing with the long short-term memory (LSTM), CNN takes much less time for the training but has way too many parameters.

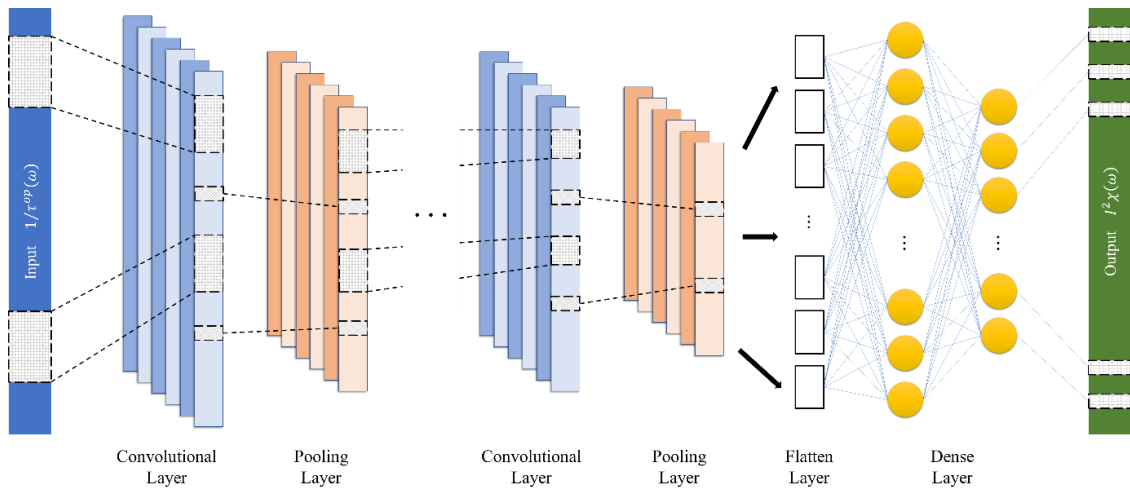

**Figure S1.** A schematic diagram of the CNN with the convolutional and pooling layers for deep learning.

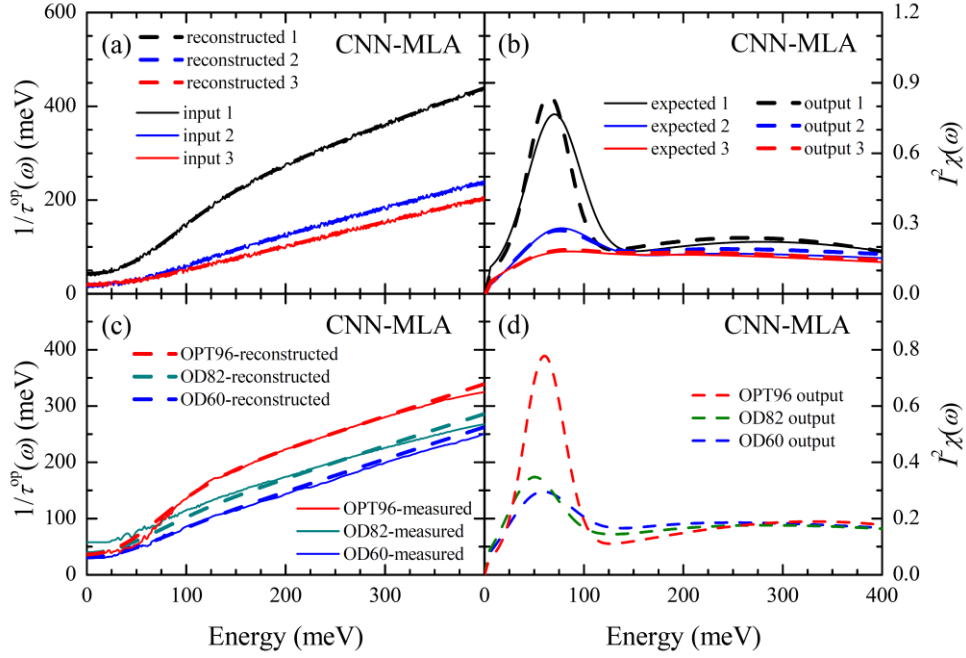

**Figure S2.** (a) Input data (solid lines) and reconstructed ones (dashed lines) using the CNN-MLA. (b) Comparison of resulting  $I^2\chi(\omega)$  (dashed lines) obtained using CNN-MLA with the expected (or original)  $I^2\chi(\omega)$  (solid lines). (c) Measured optical scattering rates of Bi-2212 samples (OPT96, OD82, and OD60: solid lines) and the corresponding optical scattering rates (dashed lines) reconstructed by using the CNN-MLA. (d) Resulting glue functions obtained from the measured optical scattering rates by using the CNN-MLA.

When we train the CNN model, we used the same training data, which we used to train the LSTM model (see in the main text). The training took  $\sim 6.5$  h on an NVIDIA GeForce RTX 2070 Super graphics processing unit (GPU) and the processing time for obtaining an output with the trained CNN model was 4 ms. The test mean-square-error (MSE) is  $3.67 \times 10^{-4}$ , which is roughly three times larger than that of the LSTM-MLA ( $1.14 \times 10^{-4}$ ). In Fig. S2, we show results of evaluations (a and b) and applications (c and d) for the three measured optical spectra of  $\text{Bi}_2\text{Sr}_2\text{CaCu}_2\text{O}_{8+\delta}$  (OPT976, OD82, and OD60) in the main text. Fig. S2(a) shows that three input data (solid) and the corresponding input data (dashed) reconstructed using the CNN machine learning approach (CNN-MLA). They agree well each other. Fig. 2(b) shows the resulting glue functions ( $I^2\chi(\omega)$ ) (dashed lines) obtained from the three input  $1/\tau^{\text{op}}(\omega)$  using the CNN-MLA and the original  $I^2\chi(\omega)$  (solid lines) used for generating the input data. These evaluations show that the training is reasonably well-performed. Fig. S2(c) shows the three experimentally measured optical scattering rates (solid lines) of OPT96, OD82, and OD60 of Bi-2212 at 100 K and the corresponding optical scattering rates (dashed lines) reconstructed using the CNN-MLA. Fig. 2S(d) shows the resulting glue functions ( $I^2\chi(\omega)$ ) obtained from the three measured optical scattering rates using the CNN-MLA. Comparing

with results obtained using the LSTM-MLA, we concluded that the LSTM-MLA is superior to the CNN-MLA; the LSTM provides a stable and consistent learning results and less MSE, even though its training time is three times longer than that of the CNN-MLA (6.5 h for CNN and 19 h for LSTM with an NVIDIA GeForce RTX 2070 Super GPU). Because the data processing times for each input data file are similar for both MLAs (4 ms for CNN and 5 ms for LSTM), we used the LSTM-MLA for our study.

### Training-data set (or model) dependency of MLA

We generated the training data set of  $1/\tau^{\text{op}}(\omega)$  using Eq. (2) and Eq. (3). But, in this case, we excluded the Gaussian term (or the first term) in the model  $I^2\chi(\omega)$  (see Eq. (3)). We prepared 100,000 + 10,000 training and test data of  $1/\tau^{\text{op}}(\omega)$  with this revised model – the first term excluded – by systematically changing the parameters in Eq. (3). We trained the LSTM neural network with this revised dataset. The test mean-square-error (MSE) using the remaining 10,000 data is  $1.10 \times 10^{-6}$ , which is around one hundredth of that ( $1.14 \times 10^{-4}$ ) of the previous LSTM-MLA trained with the original training dataset, indicating that the simpler form of  $I^2\chi(\omega)$  gives the lower test MSE. Fig. S3(a) shows three input data (solid lines) containing random noise with the amplitude of 10 meV and the corresponding input data (dashed lines) reconstructed using the LSTM-MLA. As we expected from the test MSE, the input data and reconstructed ones agree very well each other. Fig. 3(b) shows the resulting output  $I^2\chi(\omega)$  obtained from the three input  $1/\tau^{\text{op}}(\omega)$  using the LSTM-MLA (dashed lines) and the expected (or original)  $I^2\chi(\omega)$  (solid lines) used for generating the input data. Again, the resulting output  $I^2\chi(\omega)$  shows excellently match with the expected  $I^2\chi(\omega)$ .

Further, we applied the LSTM-MLA to the measured spectra of Bi-2212 (OPT96, OD82, and OD60). Fig. S3(c) shows the three experimental spectra (solid lines) and the corresponding ones (dashed lines) reconstructed using the LSTM-MLA; we observe some disagreements between them. From a close examination, we observe that the reconstructed ones cannot capture the sharp kink features of the OPT96 curve located near 50 and 120 meV. Fig. 3(d) shows resulting output  $I^2\chi(\omega)$  obtained from the three input spectra  $1/\tau^{\text{op}}(\omega)$  using the LSTM-MLA. The resulting  $I^2\chi(\omega)$  are significantly different from the corresponding results in the main text (see Fig. 4(b)). These results indicate that the training data generated from the model glue function ( $I^2\chi(\omega)$ ) is not rich enough to account for the data manifold appropriate to obtain a reasonable output glue function from the measured spectra of Bi-2212. One needs

to elaborate the model glue function for training and obtaining a reliable output glue function. For doing this, in the main text, we utilized the shapes of the glue functions obtained from the measured spectra using the maximum entropy method (MEM); we used Eq. (3) for the model  $I^2\chi(\omega)$ .

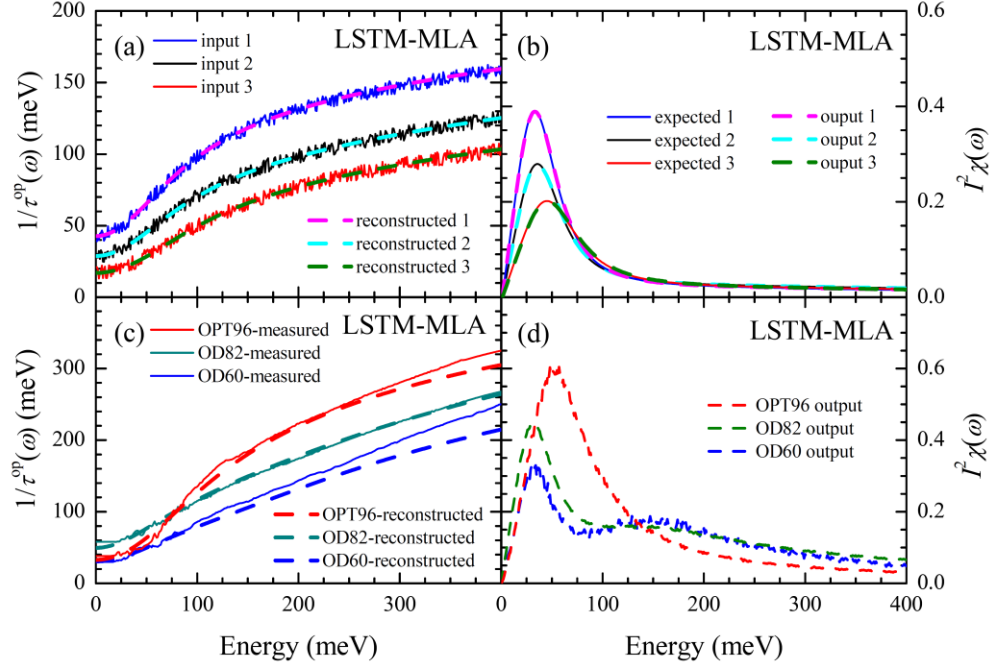

**Figure S3.** (a) Input data (solid lines) and reconstructed ones (dashed lines) using the LSTM -MLA. (b) Comparison of the resulting  $I^2\chi(\omega)$  (dashed lines) obtained using the LSTM-MLA with the expected (or original)  $I^2\chi(\omega)$  (solid lines). (c) Measured optical scattering rates of Bi-2212 samples (OPT96, OD82, and OD60: solid lines) and the corresponding spectra (dashed lines) reconstructed using the LSTM-MLA. (d) Resulting glue functions obtained from the measured optical scattering rates using the LSTM-MLA.
